# Supplementary material for: Empirical Analysis of a Segmentation Foundation Model in Prostate Imaging
Source: arXiv:2307.03266 source file (2023-10-02)
Supplement: Supplementary file 1 [file Appendix-arxiv.pdf]

# Appendix

## 1 Implementation details of nnUNet

We used the two 2D nnUNet models with the different number of parameters. The first nnUNet (nnUNet-original) follows the automatic network configuration of original paper [1] and the second nnUNet model (nnUNet-small) is a smaller network capacity that matches to the size of the UniverSeg model (1.2M parameters) . For our nnUNet-small implementation had 1.3M learnable parameters by setting the base number of feature maps to 16 and the maximum number of features to 96.

For both models, we followed the training parameters provided in the original nnUNet paper [1]. A five-fold cross validation is applied. Each model is trained from a random initialization using heavy data augmentation and ensembling. The data augmentation includes rotation, scaling, mirroring, Gaussian Noise, Gaussian Blur, brightness, contrast, simulation of low resolution, and gamma augmentation. The models are trained for 1,000 epochs using the sum of cross-entropy and Dice loss. The further details of augmentation and training schedule parameters can be found in Supplementary Note 4 and Method Section of the nnUNet paper [1].

## 2 Table

| | Method | $N=1$ | $N=2$ | $N=5$ | $N=10$ |
|---|---|---|---|---|---|
| | | **ROI: TZ** | | | |
| nnUNet-Orig | wo-augmentation | $0.612 \pm 0.051$ | $0.762 \pm 0.035$ | $0.801 \pm 0.005$ | $0.818 \pm 0.010$ |
| | fold-0 | $0.581 \pm 0.064$ | $0.754 \pm 0.028$ | $0.787 \pm 0.010$ | $0.814 \pm 0.008$ |
| | fold-1 | $0.603 \pm 0.055$ | $0.757 \pm 0.029$ | $0.783 \pm 0.015$ | $0.807 \pm 0.018$ |
| | fold-2 | $0.609 \pm 0.032$ | $0.750 \pm 0.033$ | $0.786 \pm 0.009$ | $0.807 \pm 0.013$ |
| | fold-3 | $0.605 \pm 0.053$ | $0.756 \pm 0.033$ | $0.793 \pm 0.011$ | $0.812 \pm 0.009$ |
| | fold-4 | $0.624 \pm 0.037$ | $0.751 \pm 0.036$ | $0.794 \pm 0.003$ | $0.811 \pm 0.009$ |
| | default | $0.614 \pm 0.049$ | $0.764 \pm 0.034$ | $0.803 \pm 0.006$ | $0.821 \pm 0.010$ |
| nnUNet-Small | wo-augmentation | $0.601 \pm 0.065$ | $0.757 \pm 0.033$ | $0.797 \pm 0.006$ | $0.812 \pm 0.010$ |
| | fold-0 | $0.579 \pm 0.073$ | $0.747 \pm 0.031$ | $0.780 \pm 0.007$ | $0.805 \pm 0.010$ |
| | fold-1 | $0.594 \pm 0.052$ | $0.750 \pm 0.029$ | $0.776 \pm 0.018$ | $0.804 \pm 0.014$ |
| | fold-2 | $0.606 \pm 0.047$ | $0.749 \pm 0.030$ | $0.787 \pm 0.008$ | $0.797 \pm 0.018$ |
| | fold-3 | $0.579 \pm 0.077$ | $0.748 \pm 0.032$ | $0.785 \pm 0.011$ | $0.807 \pm 0.011$ |
| | fold-4 | $0.603 \pm 0.048$ | $0.742 \pm 0.040$ | $0.786 \pm 0.004$ | $0.803 \pm 0.009$ |
| | default | $0.599 \pm 0.066$ | $0.759 \pm 0.033$ | $0.800 \pm 0.006$ | $0.814 \pm 0.011$ |
| UniverSeg | all | $0.632 \pm 0.046$ | $0.717 \pm 0.010$ | $0.738 \pm 0.015$ | $0.745 \pm 0.015$ |
| | random | – | – | $0.733 \pm 0.015$ | $0.739 \pm 0.014$ |
| | random+5 ensemble | – | – | $0.736 \pm 0.015$ | $0.743 \pm 0.014$ |
| | z-weighted | – | – | $0.740 \pm 0.012$ | $0.751 \pm 0.015$ |
| | z-weighted+5 ensemble | – | – | $0.743 \pm 0.012$ | $0.754 \pm 0.015$ |
| | | **ROI: PZ** | | | |
| nnUNet-Orig | wo-augmentation | $0.369 \pm 0.107$ | $0.587 \pm 0.040$ | $0.640 \pm 0.041$ | $0.702 \pm 0.017$ |
| | fold-0 | $0.380 \pm 0.109$ | $0.592 \pm 0.022$ | $0.635 \pm 0.037$ | $0.696 \pm 0.019$ |
| | fold-1 | $0.373 \pm 0.090$ | $0.535 \pm 0.076$ | $0.630 \pm 0.033$ | $0.700 \pm 0.020$ |
| | fold-2 | $0.360 \pm 0.122$ | $0.589 \pm 0.029$ | $0.621 \pm 0.028$ | $0.695 \pm 0.010$ |
| | fold-3 | $0.361 \pm 0.094$ | $0.578 \pm 0.046$ | $0.654 \pm 0.044$ | $0.682 \pm 0.026$ |
| | fold-4 | $0.385 \pm 0.099$ | $0.593 \pm 0.027$ | $0.620 \pm 0.057$ | $0.697 \pm 0.015$ |
| | default | $0.368 \pm 0.111$ | $0.589 \pm 0.041$ | $0.644 \pm 0.042$ | $0.706 \pm 0.018$ |
| nnUNet-Small | wo-augmentation | $0.335 \pm 0.120$ | $0.569 \pm 0.047$ | $0.627 \pm 0.050$ | $0.694 \pm 0.016$ |
| | fold-0 | $0.344 \pm 0.127$ | $0.585 \pm 0.039$ | $0.621 \pm 0.033$ | $0.692 \pm 0.015$ |
| | fold-1 | $0.370 \pm 0.103$ | $0.525 \pm 0.073$ | $0.624 \pm 0.048$ | $0.679 \pm 0.016$ |
| | fold-2 | $0.336 \pm 0.129$ | $0.554 \pm 0.034$ | $0.611 \pm 0.042$ | $0.686 \pm 0.021$ |
| | fold-3 | $0.338 \pm 0.094$ | $0.563 \pm 0.045$ | $0.625 \pm 0.053$ | $0.678 \pm 0.015$ |
| | fold-4 | $0.335 \pm 0.108$ | $0.574 \pm 0.044$ | $0.619 \pm 0.054$ | $0.688 \pm 0.023$ |
| | default | $0.333 \pm 0.122$ | $0.572 \pm 0.048$ | $0.633 \pm 0.049$ | $0.699 \pm 0.016$ |
| UniverSeg | all | $0.478 \pm 0.056$ | $0.570 \pm 0.014$ | $0.650 \pm 0.019$ | $0.672 \pm 0.012$ |
| | random | – | – | $0.638 \pm 0.019$ | $0.657 \pm 0.011$ |
| | random+5 ensemble | – | – | $0.647 \pm 0.019$ | $0.668 \pm 0.012$ |
| | z-weighted | – | – | $0.640 \pm 0.018$ | $0.664 \pm 0.014$ |
| | z-weighted+5 ensemble | – | – | $0.647 \pm 0.018$ | $0.673 \pm 0.015$ |

**Table 1.** 2D Dice scores from the ablation study conducted for transitional zone (TZ) and peripheral zone (PZ) segmentation tasks

## References

1. Isensee, F., Jaeger, P.F., Kohl, S.A., Petersen, J., Maier-Hein, K.H.: nnu-net: a self-configuring method for deep learning-based biomedical image segmentation. Nature methods **18**(2), 203–211 (2021)
